# Supplementary material for: Self-detecting gate-tunable nanotube paddle resonators
Source: arXiv:0809.0372 source file (2008-09-02)
Supplement: Supplementary file 1 [file suppinfo.pdf]

**Supporting online material**

# Supporting online material

**Supplementary information on device parameters, the ac conductance of the nanotubes, the peak shape of AM actuated mechanical resonators used as frequency mixers, the derivation of the flexural spring constant and information on the finite element simulations discussed in the main paper.**

### Ac conductance of the paddle resonator

The conductance of a suspended carbon nanotube (CNT) resonator driven with an ac gate voltage is influenced by charging effects and strain in the nanotubes. These ac conductance contributions are discussed in more detail in this section.

The conductance of a semiconducting nanotube resonator at room temperature, electrostatically coupled to a gate electrode with capacitance $C_g$ and dc gate voltage $V_g^{dc}$, depends on the induced charge, an effect that enables the use of CNTs as transistors [1]. This means that an ac voltage applied to the back gate electrode leads to an (electrical) ac conductance contribution $G_{el}^{ac} = \frac{\partial G}{\partial V_g} V_g^{ac}$, where $\frac{\partial G}{\partial V_g}$ is the transconductance of the nanotube [2, 3]. Besides this well known transistor effect, the induced charge can also change when the nanotube displaces. A change in gate capacitance $C_g^{ac}$ either due to a displacement $y^{ac}$ or rotation of the paddle by angle $\theta^{ac}$ (around the nanotube axis), modulates the charge on the nanotube, which leads to a conductance contribution [2, 3]:

$$G_{mQ}^{ac} = \frac{\partial G}{\partial V_g} \frac{V_g^{dc}}{C_g} \left( \frac{\partial C_g}{\partial y} y^{ac} + \frac{\partial C_g}{\partial \theta} \theta^{ac} \right). \quad \text{(S1)}$$

Note that the rotation of the paddle only significantly alters the capacitance if the paddle offset $\delta > 0$ (see Fig 1(a) of the main text).

In addition to capacitively induced conductance changes, piezoresistive effects can play a role [4]. A displacement or a twist of the nanotube, induces longitudinal strain $\epsilon_L$ or torsional strain $\gamma$ respectively. Strain can change the bandstructure of certain nanotubes [5], which results in a modification of the nanotube resistance. The ac conductance due to piezoresistive effects is described by:

$$G_{m\epsilon}^{ac} = \frac{\partial G}{\partial \epsilon_L} \frac{\partial \epsilon_L}{\partial y} y^{ac} + \frac{\partial G}{\partial \gamma} \frac{\partial \gamma}{\partial \theta} \theta^{ac}. \quad \text{(S2)}$$

The dependence of the conductance $G(\epsilon_L, \gamma)$ of a nanotube on strain is found in Ref. [4, 5], while the expressions for $\partial \epsilon_L / \partial y$ and $\partial \gamma / \partial \theta$ will be published elsewhere.

Since both mechanisms can occur simultaneously, a priori, no distinction can be made between the contributions. The ac conductance is thus described by an electric ($G_{el}^{ac}$) and a mechanical ($G_{mech}^{ac} = G_{mQ}^{ac} + G_{m\epsilon}^{ac}$) conductance contribution. When a mechanical resonance is approached, the nanotube and paddle oscillation amplitude increases significantly. For flexural modes $y^{ac}$ increases in magnitude, while for torsional modes $\theta^{ac}$ becomes larger. Both contributions to the mechanical conductance changes can be summarized as:

$$G_{mech}^{ac} = \frac{dG}{dy} y^{ac} + \frac{dG}{d\theta} \theta^{ac}, \quad \text{(S3)}$$

where $\frac{dG}{dy}$ and $\frac{dG}{d\theta}$ are the flexural and torsional transconductance respectively, and can be obtained from Eqs. S1 and S2.

TABLE SI: Estimates of the physical parameters of device 1 and 2. The parameters are the radius of the nanotube $r$, the width of the paddle (perpendicular to the nanotube) $w_p$, the length of the paddle (parallel to the nanotube) $L_p$, the offset $\delta$ of the center of mass of the paddle from the nanotube axis and the length of the nanotube sections $L_1$ and $L_2$ respectively. The estimates are obtained from either atomic force microscope (AFM) experiments (†) or SEM images (‡).

| Device: | 1 | 2 |
|---|---|---|
| $r^\dagger$ (nm) | 1.43 | 2.16 |
| $w_p^\ddagger$ (nm) | 232 | 206 |
| $L_p^\ddagger$ (nm) | 84 | 116 |
| $\delta^\ddagger$ (nm) | 45 | 37 |
| $L_1^\ddagger$ (nm) | 600 | 408 |
| $L_2^\ddagger$ (nm) | 600 | 487 |

### Lock-in phase and amplitude for the AM technique

The shape of the amplitude and phase of the downmixed lock-in amplifier current $I^{LIA} = I^{ac} \cos(\omega_m t + \xi)$ at the (angular) modulation frequency $\omega_m$, are analyzed in this section.

TABLE SII: With the estimates given in table SI, the moment of inertia $I_p$ of the paddle around the nanotube and the total torsional spring constant $k$ are calculated.

| Device: | 1 | 2 |
|---|---|---|
| $I_p$ ($10^{-32}$ kg m$^2$) | 3.42 | 3.21 |
| $k$ ($10^{-18}$ Nm/rad) | 4.48 | 31.57 |
| $k/I_p$ ($10^{14}$ s$^{-2}$) | 1.31 | 9.83 |

Since the ac gate voltage in the experiments is much smaller than the dc voltage, the force/torque acting on the paddle resonator has a dc component $\propto (V_g^{dc})^2$ and an ac component $\propto 2V_g^{dc}V_g^{ac}\cos(\omega t)$. The nanotube resonator can be described as a damped driven harmonic oscillator [3], with (normalized) response function $H(\omega) = 2\omega_0^2/Q \times 1/(\omega_0^2 - \omega^2 - i2\omega\omega_0/Q)$, resonance frequency $\omega_0$, quality factor $Q$ and phase $\zeta = \angle H(\omega)$ [7], driven at frequency $\omega$. The ac conductance of the nanotube resonator at frequency $\omega$ due to the actuation voltage on the gate electrode of the nanotube can be described by [3]:

$$G^{ac}(\omega) = G_{el}^{ac}\cos(\omega t) + G_{mech}^{ac}|H(\omega)|\cos(\omega t + \zeta(\omega)), \quad \text{(S4)}$$

where $G_{el}^{ac} = \frac{\partial G}{\partial V_g^{dc}} V_g^{ac}$ is the change in conductance due to electrical effects, and $G_{mech}^{ac}$ is the mechanical contribution due to vibrations of the nanotube, which can be caused by either capacitance changes [2, 3] or piezoresistive effects [4]. .

Since the actuation voltage is 100 % AM modulated and the driving force is proportional to $V_g^{dc}V_g^{ac}$, the ac driving force has the form:

$$F \propto (1 + \cos(\omega_m t))\cos(\omega_c t), \quad \text{(S5)}$$

where $\omega_c$ is the carrier frequency and $\omega_m$ is the modulation frequency. The mechanical response (when there is a non-zero ac displacement $y^{ac}$ and/or torsional angle $\theta^{ac}$) of the AM driven resonator is then:

$$\begin{aligned} y^{ac}, \theta^{ac} \propto\; & |H(\omega_c)|\cos(\omega_c t + \zeta(\omega_c)) \quad \text{(S6)} \\ & + \frac{1}{2}|H(\omega_c + \omega_m)|\cos((\omega_c + \omega_m)t + \zeta(\omega_c + \omega_m)) \\ & + \frac{1}{2}|H(\omega_c - \omega_m)|\cos((\omega_c - \omega_m)t + \zeta(\omega_c - \omega_m)). \end{aligned}$$

Using Eq. S4 for each of the spectral components of equation S6, the total ac conductance of the AM driven resonator therefore is:

$$G_{tot}^{ac} = G^{ac}(\omega_c) + G^{ac}(\omega_c + \omega_w) + G^{ac}(\omega_c - \omega_w). \quad \text{(S7)}$$

The device is biased with an AM signal that is spectrally *identical* to the ac gate-voltage:

$$\begin{aligned} V_b^{ac} &= V_b^{ac}(\cos(\omega_c t + \phi) \\ &+ \frac{1}{2}\cos((\omega_c + \omega_m)t + \phi) \\ &+ \frac{1}{2}\cos((\omega_c - \omega_m)t + \phi)), \quad \text{(S8)} \end{aligned}$$

where $\phi$ is a phase difference between the bias and gate voltage.

The resulting current flowing through the nanotube is the product of Eq. S8 and the ac conductance described in Eq. S7, containing 10 spectral terms. Since the lock-in amplifier uses the modulation frequency $\omega_m$ as a reference, we only consider spectral components at the modulation frequency. The measured lock-in signal $I^{ac}\cos(\omega_m t + \xi)$ can be described by an amplitude $I^{ac}$ and phase $\xi$ that can be expressed in terms of the bias and the ac conductance:

$$I^{ac} = \frac{1}{4}V_b^{ac}\sqrt{a^2 + b^2} \quad \text{(S9)}$$

$$\xi = \frac{1}{2}\arccos\left(\frac{a^2 - b^2}{a^2 + b^2}\right), \quad \text{(S10)}$$

where

$$\begin{aligned} a &= 4G_{el}^{ac}\cos(\phi) + G_{mech}^{ac}[2|H(\omega_c)|\cos(\phi - \zeta(\omega_c)) \\ &+ |H(\omega_c + \omega_m)|\cos(\phi - \zeta(\omega_c + \omega_m)) \\ &+ |H(\omega_c - \omega_m)|\cos(\phi - \zeta(\omega_c - \omega_m))] \\ b &= G_{mech}^{ac}[|H(\omega_c - \omega_m)|\sin(\phi - \zeta(\omega_c - \omega_m)) \\ &- |H(\omega_c + \omega_m)|\sin(\phi - \zeta(\omega_c + \omega_m))]. \end{aligned}$$

Note that the lock-in amplitude of the peak $I^{ac}$ is proportional to the bias amplitude $V_b$, and that the lock-in phase $\xi$ is independent of the bias amplitude. When the modulation frequency $\omega_m = 0$, the amplitudes and phases of the individual cosines in coefficients $a$ and $b$ become equal, and the phase no longer contains information on the mechanical resonance (comparable to the traditional frequency mixing scheme [3]). An example of a resonance peak shape and the corresponding phase is shown in Fig. S1 for typical values of our devices.

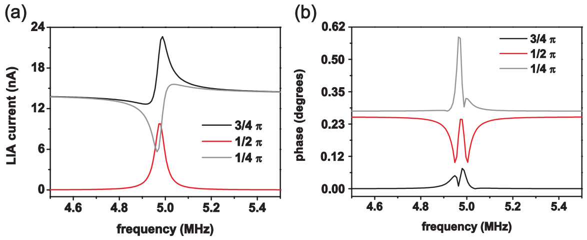


FIG. S1: (a) Resonance shape as a function of carrier frequency (with $\omega_m = 500$ Hz), for a resonator with eigenfrequency $\omega_0 = 5$ MHz and $Q = 200$, with bias voltage 100 mV and conductance amplitudes $G_{el}^{ac} = 0.2 \times 10^{-6}$ and $G_{mech}^{ac} = -1 \times 10^{-7}$ for $\phi = \frac{1}{4}\pi$, $\frac{1}{2}\pi$ and $\frac{3}{4}\pi$. (b) Lock-in phase as a function of the carrier frequency, for $\phi = \frac{1}{4}\pi$, $\frac{1}{2}\pi$ and $\frac{3}{4}\pi$ (offset for clarity).

### Flexural spring constant of a nanotube section

To determine the flexural spring constant of the nanotube sections, we need to know the force acting on the nanotube via the paddle, and the displacement at $x$=$L$ (paddle-nanotube interface). The latter is determined by calculating the incremental displacement of the nanotube $y(x)$. To obtain an expression for $y(x)$, we use a similar

approach as in Ref. [6]. The incremental displacement is described by a purely static form of a Euler-Bernoulli equation with an extra tension term:

$$EI\frac{d^4y(x)}{dx^4} - T_{dc}\frac{d^2y(x)}{dx^2} = 0, \quad \text{(S11)}$$

where the tension $T_{dc}$ is solved self-consistently from [3]

$$T_{dc} = \frac{EA}{2L}\int_0^L \left(\frac{dy(x)}{dx}\right)^2 dx. \quad \text{(S12)}$$

In these equations $I$, $A$ and $L$ are the second moment of area of the nanotube along the tube axis ($\pi r^4/4$), the nanotube cross-section area and the length of the tube between the clamping point of the resonator and the nanotube-paddle interface respectively. Note that in contrast to Ref. [6], Eq. S11 does not have a force term on the right side because we assume that the electrostatic force acting on the paddle is felt by the nanotube only at the nanotube-paddle interface, and thus has to be included in the boundary conditions at $x = L$.

The boundary conditions on the displacement of the tube section described by Eq. S11 therefore are:

$$y(0) = 0 \quad \text{(S13)}$$
$$y^{'}(0) = 0 \quad \text{(S14)}$$
$$y^{'}(L) = 0 \quad \text{(S15)}$$
$$y^{'''}(L) = \frac{F}{EI}, \quad \text{(S16)}$$

where the first two conditions describe the clamping point of the resonator, the third condition forces the paddle to only displace in the direction of the force acting on it. The fourth condition describes the moment induced on the tube section due to the force acting at point $x$=$L$.

To facilitate the analysis of the differential Eq. S11, we convert all the variables to dimensionless units. Combining the solution of Eqs. S11 and S13-S16 with Eq. S12, results in a self-consistent equation for tension in the nanotube versus the force acting on the nanotube. Three regimes can be distinguished; a weak tension regime, a strong regime and an intermediate regime. This weak- to strong tension transition is similar to normal suspended nanotubes [3, 6]. For the weak tension regime, the tension is proportional to $F^2$. The shape of the nanotube section is shown in figure S2. For the strong tension regime the tension is proportional to $F^{\frac{2}{3}}$. The intermediate regime can only be calculated numerically.

Now that the incremental displacement at each of the nanotube sections is known, as a function of the force (via the tension) acting on the paddle, we can determine the spring constant $\kappa$ of a nanotube section (in the displacement direction), by dividing the force $F$ by the displacement $y(L)$ at $x$=$L$. At zero gate voltage (i.e. when $T \rightarrow 0$), the spring constant of an individual nanotube section is equal to $\frac{12EI}{L^3}$. At higher gate voltages, the spring constant becomes stiffer, leading to higher flexural eigenfrequencies.

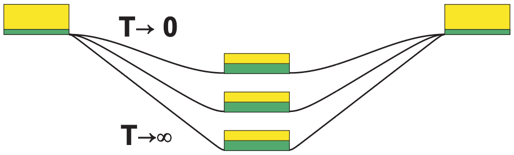


FIG. S2: Flexural displacement of the paddle and its CNT springs for three tension regimes.

**Finite-element simulations**

To determine the capacitance coefficients $B_0$, $B_1$ and $B_2$ described in the main paper, 2D finite element simulations (FEM) are used to calculate the potential landscape around a metal paddle (grounded) with a torsional angle $\theta$ above a back-gate electrode (potential 1 V). A result of such a calculation result is shown in figure S3 for $\theta = 45$. The capacitance between the paddle and the back-gate

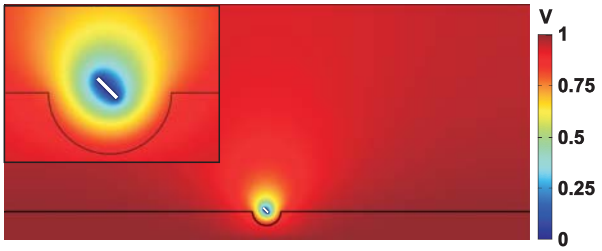


FIG. S3: Electrostatic potential landscape of a paddle (white) at a torsional angle of 45 degrees, calculated with FEM simulations. Inset: zoom of the potential around the paddle (white).

can then be calculated for different torsional angles $\theta$. For devices 1 and 2 described in the main paper (Fig. S4 (a) and (b)), the capacitance as a function was calculated using the parameters of table SI. The capacitance $C_g$ in

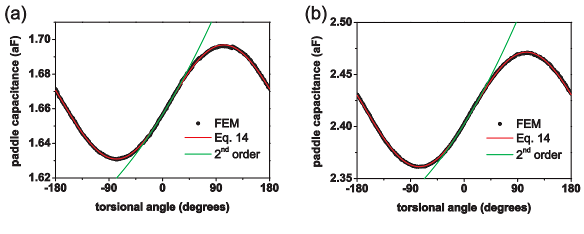


FIG. S4: Capacitance between the paddle and the back-gate electrode for $-180 < \theta < 180$, calculated with FEM for devices 1 (a) and 2 (b). To these FEM data points, Eq. 14 is fit (red lines). A second order series approximation accurately describes the capacitance up to values of 45 degrees (green lines).

these figures can be accurately described (360 degrees) by a sine function (red lines) of the form:

$$C_g = A + D\sin(\theta - \theta_0), \qquad \text{(S17)}$$

where $A$, $D$, $\theta_0$ and $w$ are fit parameters (see table SIII). To get a value for the torque coefficients from the main paper, the sine function is expanded around $\theta = 0$ in a second order polynomial. The series expansion accurately describes the change in capacitance for angles up to 45 degrees (see green lines in Fig. S4 (a) and (b)) for both devices. The torque coefficients can then be expressed in terms of the parameters of Eq. S17: $B_0 = A - D\sin(\theta_0)$, $B_1 = D\cos(\theta_0)$ and $B_2 = D\sin(\theta_0)/2$. To obtain these torque coefficients, the polynomial is fitted to the calculated capacitance in Fig. S4 (a) and (b) (green lines) and are listed in table SIV.

TABLE SIII: Capacitance fit parameters $A$, $D$ and $\theta_0$ of equation S17

| Device: | 1 | 2 |
|---|---|---|
| $A$ ($10^{-18}$ F) | 1.66 | 2.42 |
| $D$ ($10^{-18}$ F) | 0.03 | 0.06 |
| $\theta_0$ (rad) | 0.22 | 0.26 |

TABLE SIV: Torque coefficients $B_0$, $B_1$ and $B_2$ obtained from numerical calculations, using the parameters of Eq. S17 and the corresponding second order series approximation.

| Device: | 1 | 2 |
|---|---|---|
| $B_0$ ($10^{-18}$ F) | 1.66 | 2.40 |
| $B_1$ ($10^{-20}$ F) | 3.20 | 5.32 |
| $B_2$ ($10^{-21}$ F) | 3.58 | 7.00 |

[1] Z. Yao, H. W. Ch. Postma, L. Balents and C. Dekker, Nature, **402**, 273 (1999).
[2] V. Sazonova, Y. Yaish, H. Üstünel, D. Roundy, T. A. Arias and P. L. McEuen, Nature, **431**, 284 (2004).
[3] B. Witkamp, M. Poot and H. S. J. van der Zant, Nano Lett., **6**, 2904 (2006).
[4] A. R. Hall, Michael R. Falvo, R. Superfine and S. Washburn, Nature Nanotechnology **2**, 413 - 416 (2007).
[5] T. Cohen-Karni, L. Segev, O. Srur-Lavi, S. R. Cohen and E. Joselevich, Nature Nanotechnology **1**, 36 - 41 (2006).
[6] M. Poot, B. Witkamp, M.A. Otte, H.S.J. van der Zant, Physica Status Solidi (b) **244**, 4252-4256 (2007).
[7] A. Cleland, *Foundations of Nanomechanics*, Springer (2003).
